# Supplementary material for: Density distributions and depth in flocks
Source: arXiv:1902.08181 ancillary file (2019-02-21)
Supplement: Supplementary file 1 [file SI_LewisTurner_DMBSMF_JPhysD_FirstRevisions.pdf]

# Density distributions and depth in flocks: supplemental materials

Jason M. Lewis<sup>1</sup> and Matthew S. Turner<sup>1,2</sup>

<sup>1</sup>*Centre for Complexity Science, University of Warwick, Coventry CV4 7AL, UK*

<sup>2</sup>*Department of Physics, University of Warwick, Coventry CV4 7AL, UK*

## I. DIRECTION OF MOTIONAL BIAS

Figure 1 shows the way in which the direction of motional bias is determined for a typical particle (shown for shell 0: a border particle, and analogously for others). We average over the unit vectors pointing from this particle  $i$  to its shell neighbours  $S_i$ , so this will be, on average, pointed inwards for positive values of  $f_i$ .

## II. DEFINING TOPOLOGICAL DEPTH

Figure 2 provides a step-by-step example of shell labelling in 2D. The 3D version, as used in this study, is defined analogously. By assigning each particle a label in this way, the label corresponds to the shortest path length from the border through the graph defined via the Delaunay triangulation, and we use it to determine the particles depth in the swarm topologically, giving us a broad idea as to how many particles are between each particle and the edge of the swarm.

## III. CONFIGURATIONAL SNAPSHOTS

Figure 3 shows specific instances of simulated swarms arising from the SMF model (see [26] in main text) and DMBSMF model (with SPSA fit parameters, present study). Differences exist in the local density profile for typical swarms generated by these models although this is difficult to see in a 2D projection of a 3D swarm. See main text for more details.

## IV. EVOLUTION OF FLOCK VELOCITY

Figure 4 shows the fluctuation of the flock velocity  $\underline{V}(t)$ . The system moves from a disordered initial state to an ordered one and noise-driven fluctuations in the heading of  $\underline{V}(t)$  are present for both states.

## V. FINITE SIZE STEADY-STATE

Figure 5 presents the evolution of the spatial extent of simulated DMBSMF swarms with SPSA fit parameters for initial states with varying system size, from a cube of length 1 to 1000. Regardless of initial state swarms eventually result in a cohesive steady-state of consistent size  $\bar{R}$ .

## VI. MOVIE SHOWING COLLECTIVE MOTION

Supplementary movie (shown here) shows a simulated swarm of  $N = 1500$  individuals within our distributed motional-bias strictly metric-free model with SPSA fit parameters and  $\phi_n = 0.22$ . This movie shows cross-sections of a swarm for 250 timesteps. Top-left:  $x$ - $y$ ; top-right:  $z$ - $y$ ; bottom-left:  $x$ - $z$ . The swarm evolves from an initial condition of uniformly random position distribution within a unit cube centred on the origin and uniformly random orientation, toward an ordered and cohesive steady-state with a density profile matching empirical data (see [22] in main text). Bottom-right: polarisation  $P$  of the swarm over time  $t$ . Swarm is initially disordered (low  $P$ ) and becomes more ordered (high  $P$ ) with time.

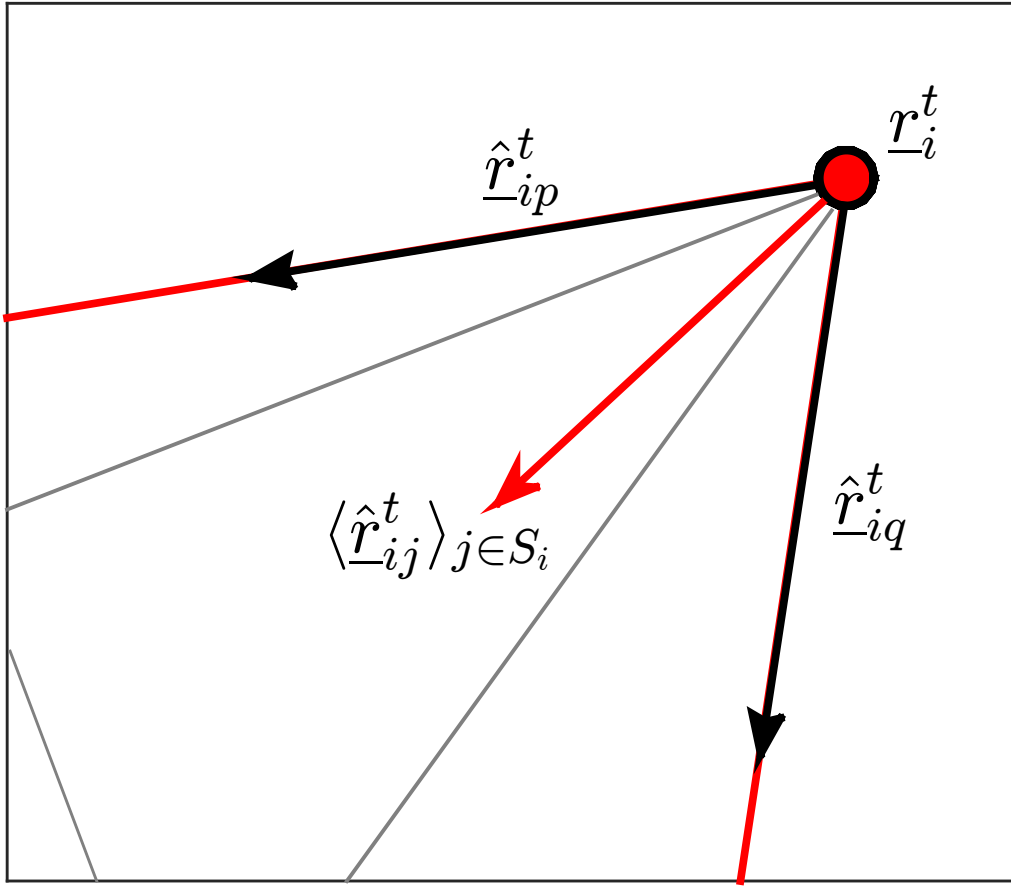

FIG. 1. Illustrative construction of bounding term for particle  $i$  at  $\underline{r}_i^t$  with shell neighbours  $p$  and  $q$ . Other neighbours (in  $B_i$  only) connected via grey lines. Effect direction (red arrow) is average of unit vectors pointing from particle  $i$  to each of the shell neighbours  $S_i = \{p, q\}$ , i.e.  $\langle \hat{r}_{ij}^t \rangle_{j \in S_i}$ .

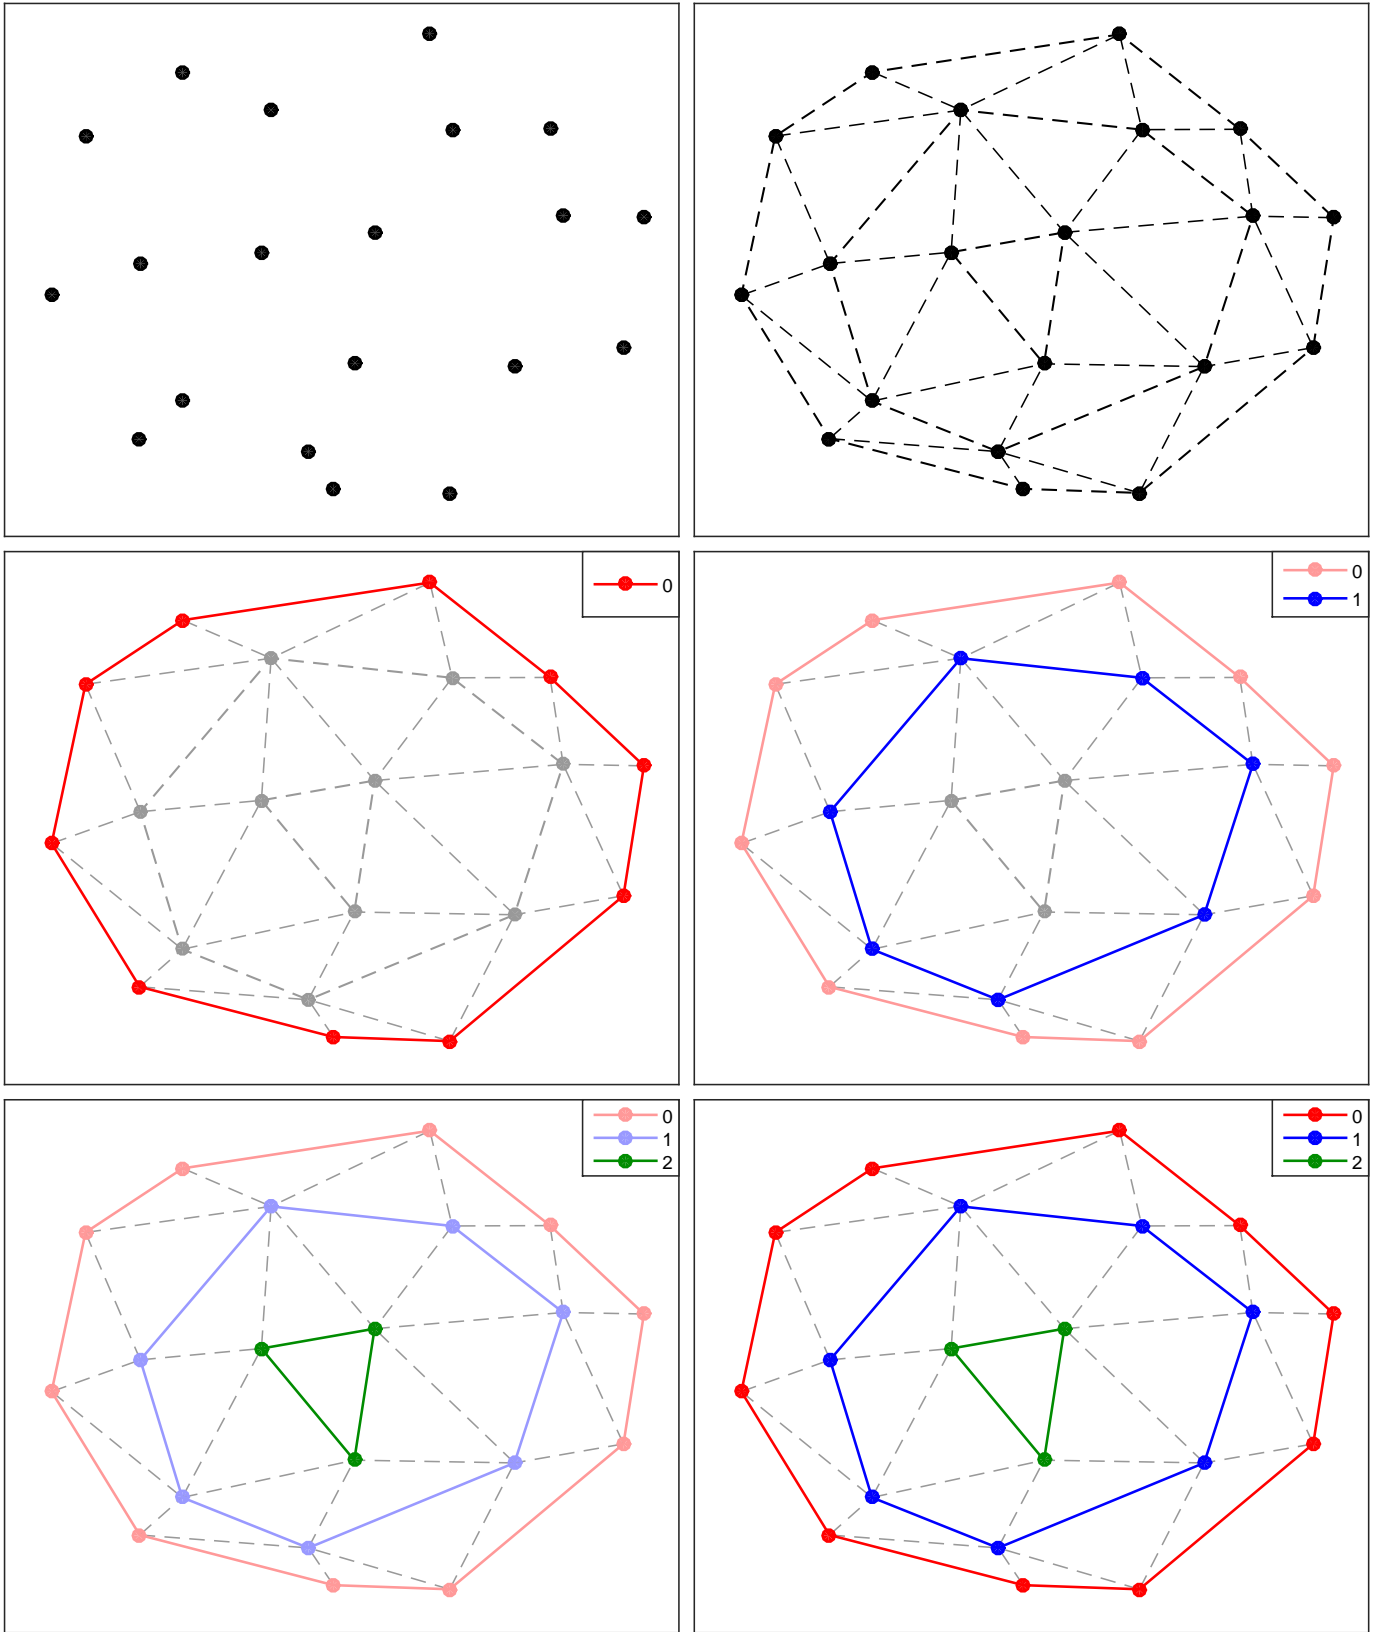

FIG. 2. Schematic of system topology (2D example): picture series illustrating successive labelling of shells from the border (shell 0) inward. (a) Black circles are particle positions at time  $t$ . (b) Black dashed lines denote edges of Delaunay graph that is dual to Voronoi tessellation of particle positions. (c) Particles on the convex hull of this point set (those which occupy infinite Voronoi cells) are defined as shell 0 (red), that is the border of the flock. (d) Moving inward, we label all particles that are connected to shell 0 particles via an edge (which are not yet labelled) as shell 1 (blue). (e) This is done iteratively, defining shell 2 particles (green) as those connected to shell 1 particles. (f) This is terminated when all particles have been labelled.

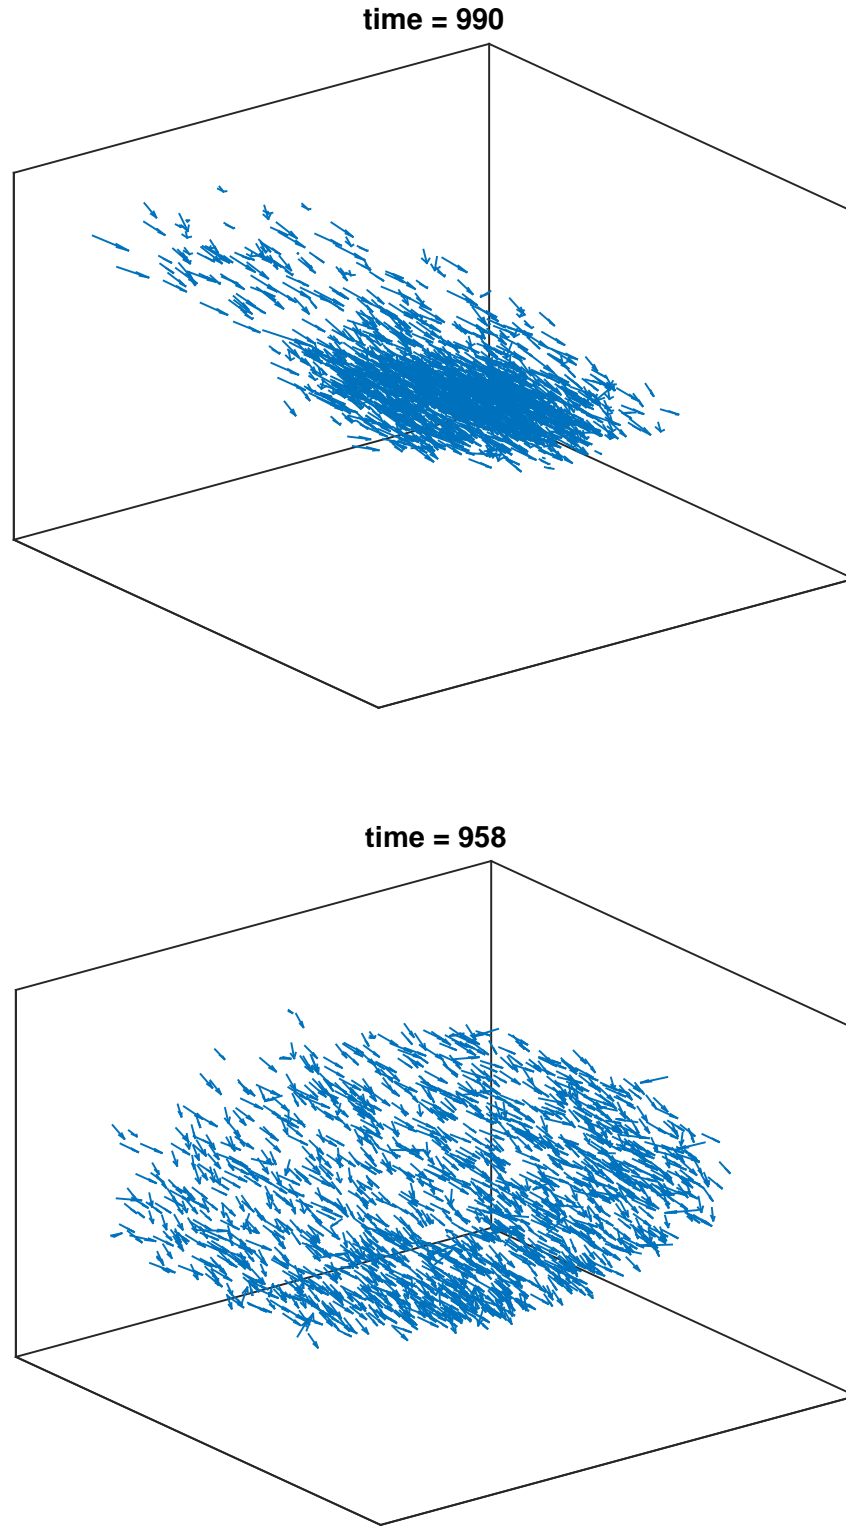

FIG. 3. Configurational snapshots of simulated swarms: (top) SMF and (bottom) SPSA fit. We observe specific regions of high density in the SMF model, however in our model tuned with fit parameters these cannot persist and density variation across aggregation is regulated similarly to that observed in the empirical study (M. Ballerini, *et al.*, Animal Behaviour, **76**, 201 (2008)).

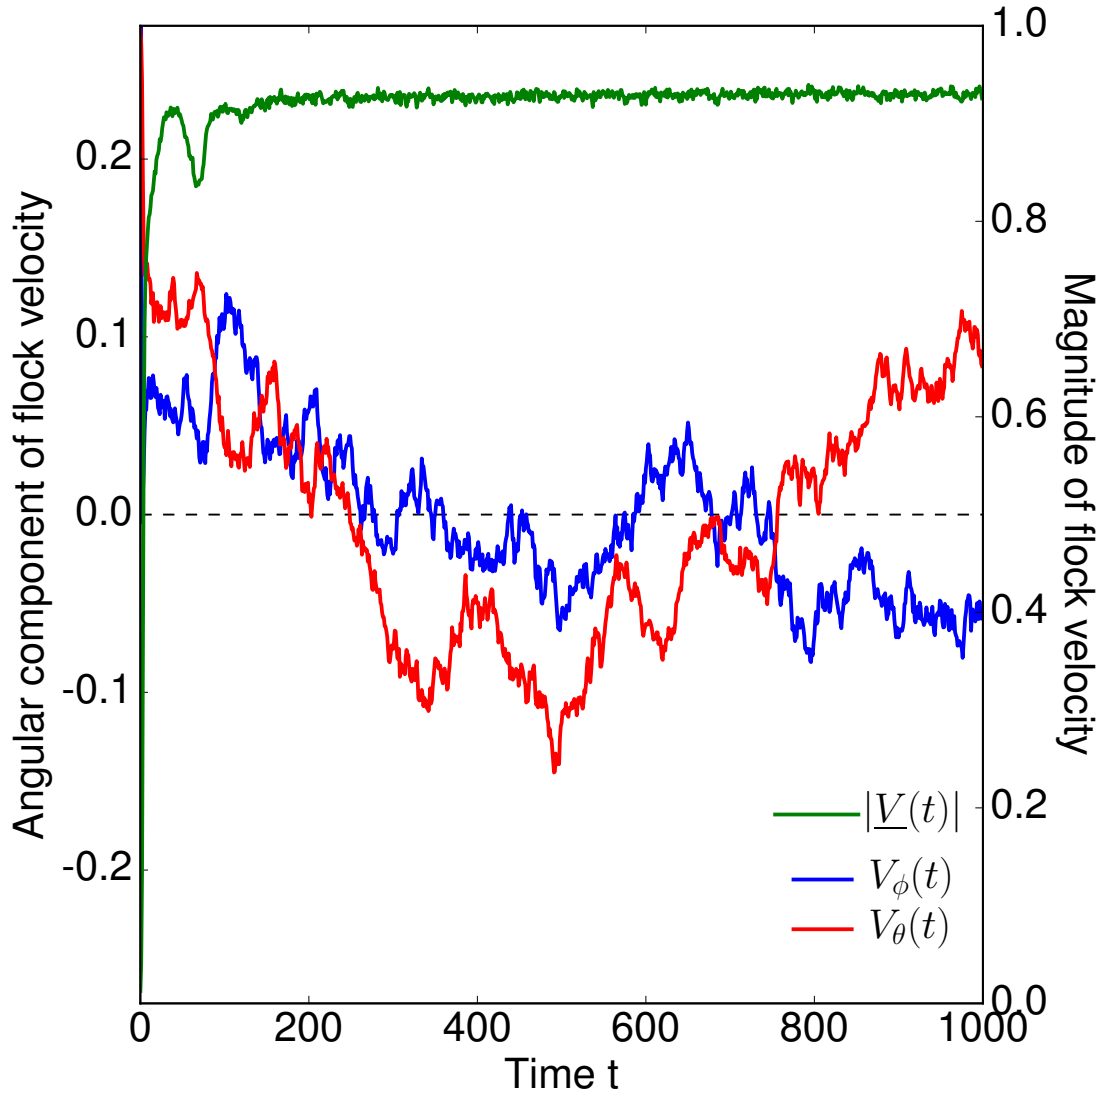

FIG. 4. Change in flock velocity over time. Simulation with SPSA fit parameters,  $\phi_n = 0.22$  and  $N = 1500$ , initialised with random positions, distributed uniformly, in a unit cube centred on the origin with random initial orientation, isotropically distributed. Flock velocity  $\underline{V} = \frac{1}{N} \sum_{i=1}^N \underline{v}_i$  grows in magnitude (green line, right axis) from close to zero, a disordered state, to close to 1 ( $\langle \underline{V}(t) \rangle = 0.92 \pm 0.06$ ), an ordered state. The angular components of  $\underline{V}$ , described in spherical polar  $\theta$  and  $\phi$ , as  $V_\phi(t)$  and  $V_\theta(t)$  (blue and red lines, left axis) respectively, are shown to fluctuate in both ordered and disordered states, driven by noise of strength  $\phi_n$ .

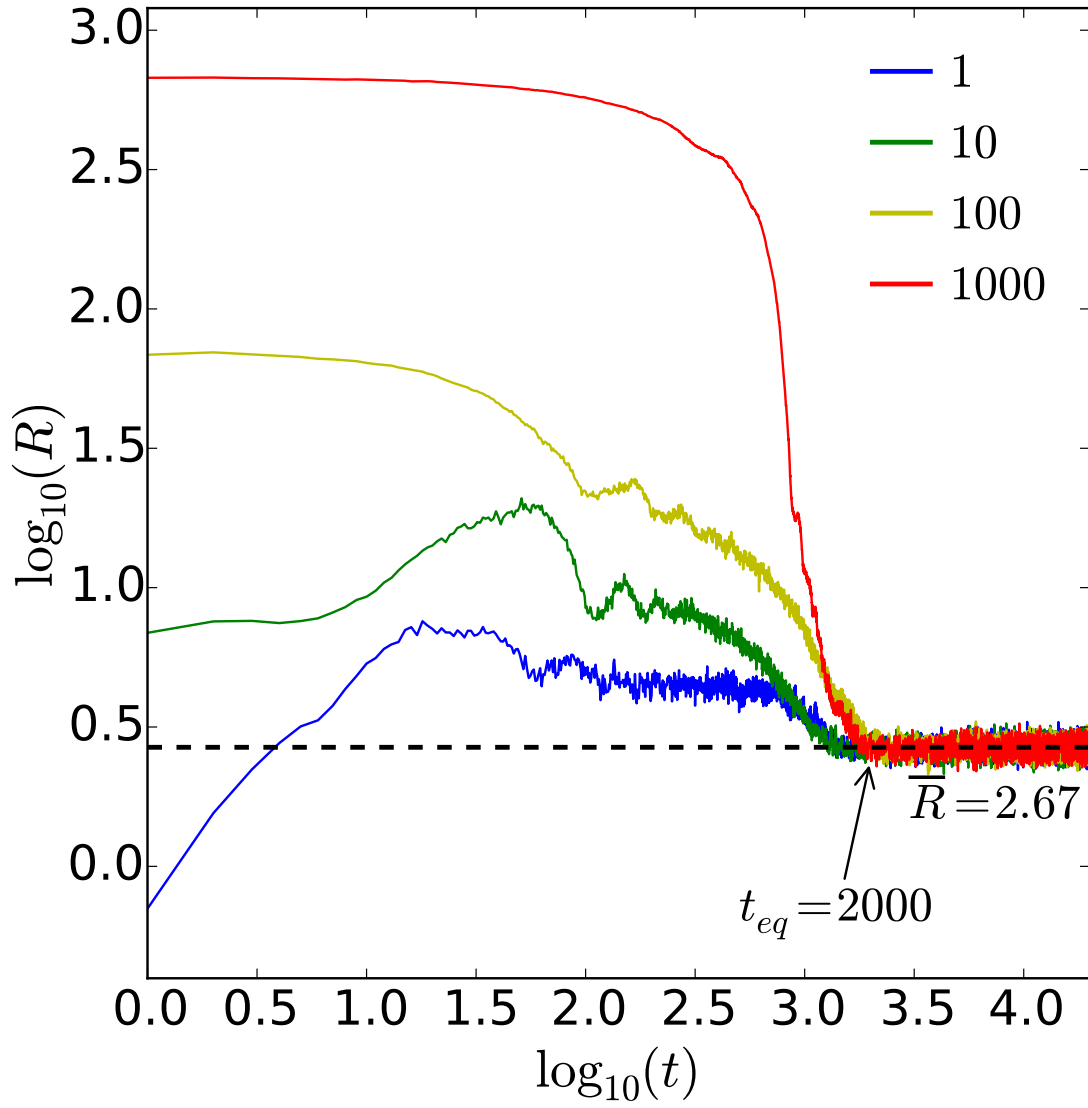

FIG. 5. Convergence to steady-state. Simulation with SPSA fit parameters,  $\phi_n = 0.22$  and  $N = 1500$ , initialised with random positions, distributed uniformly, in a cube of length  $l$  centred on origin with randomly distributed 3D orientation. Blue, green, yellow and red lines correspond to  $l = 1, 10, 100, 1000$  respectively, increasing the spatial extent of the initial state. The spatial extent  $R = \langle |r_i - r_{cm}| \rangle_{i \in C_0}$  converges to  $\bar{R}$  after equilibration time  $t_{eq}$ . A steady-state is reached asymptotically.
